# Supplementary material for: Geometrical origins of contractility in disordered actomyosin networks
Source: arXiv:1407.6693 ancillary file (2014-07-24)
Supplement: Supplementary file 1 [file Supplement.pdf]

# Geometrical origins of contractility in disordered actomyosin networks
# —
# Supporting Information

Martin Lenz[1,*]
[1] *Univ. Paris-Sud; CNRS; LPTMS; UMR 8626, Orsay 91405 France*

## I. REQUIREMENTS FOR CONTRACTILITY: NO-CONTRACTILITY PROOF

To show that a disordered network fulfilling the four conditions enumerated in the main text cannot exert net contractile force, we first express the stretching modulus $k(L)$ of a filament of arclength $L$ in terms of a dimensionless scaling function $\tilde{k}$ and the average crosslinker-to-motor distance $\xi$:

$$k(L) = k(\xi)\tilde{k}(L/\xi). \tag{S1}$$

In the rigid filament limit considered here (assumption 4. of the main text), filaments are not allowed to bend and $\mathcal{D}$ is a function of the stall force $f$, the lengths of the filament sections $\{L_i^a\}_{i,a}$ and the stretching moduli $\{k(L_i^a)\}_{i,a}$. Dimensional analysis thus reveals that the dimensionless quantity $\mathcal{D}/f\xi$ depends only on dimensionless ratios of these parameters, namely $\{L_i^a/\xi\}_{i,a}$ and $\epsilon = f/\xi k(\xi)$. In the rigid filament limit, $\epsilon$ goes to zero and we can expand $\mathcal{D}$ as

$$\mathcal{D} = f\xi\left[\tilde{\mathcal{D}}_1\left(\{L_i^a/\xi\}_{i,a}\right) + \mathcal{O}(\epsilon)\right], \tag{S2}$$

where $\tilde{\mathcal{D}}_1$ is a dimensionless function of order 1, consistent with the fact that contractile forces vanish for $f \to 0$.

We now consider the polarity-disordered character of our actomyosin network. We define polarity-reversal as the operation which transform a polar filament network configuration $\mathfrak{C}$ into a network configuration $R(\mathfrak{C})$ of identical filament positions and orientations but reversed polarities. We study polarity-reversal-symmetric networks, meaning that the probability of encountering any configuration $\mathfrak{C}$ in an experiment is equal to that of encountering $R(\mathfrak{C})$. Due to the motors' point-like nature and the infinite rigidity of the filaments, neither the motors nor the filaments move as a result of this force reversal. As a result, reversing filament polarities is mechanically equivalent to reversing the direction of the motor force, and thus $\mathcal{D}^{\mathfrak{C}}(f) = \mathcal{D}^{R(\mathfrak{C})}(-f)$. Averaging the dipole of Eq. (S2) over all possible network configurations, we thus find that the contributions of $\mathfrak{C}$ and $R(\mathfrak{C})$ cancel each other out to order $f$, implying

$$\langle\mathcal{D}\rangle = \mathcal{O}(f\xi\epsilon) = \mathcal{O}[f^2/k(\xi)] \underset{\text{rigid filament limit}}{\longrightarrow} 0. \tag{S3}$$

Therefore the motor does not exert any contractile forces on its surroundings on average.

## II. DIPOLE EXERTED BY A DEFORMABLE MOTOR

Here we calculate the average force dipole exerted by the extensible, attaching-detaching motor described by Eq. (10) of the main text. We denote by $s_1$ and $s_2$ the distance between each of the motor heads of Fig. 3(d) and the intersection between the two filaments, and write the conservation equation for the probability density $\rho(s_1, s_2; \theta)$ as

$$\partial_{s_1}(\rho v_1)+\partial_{s_2}(\rho v_2) = D(\partial_{s_1}^2\rho+\partial_{s_2}^2\rho)+k_{\text{on}}^0 e^{-E_s/k_BT}-k_{\text{off}}\rho, \tag{S4}$$

where $v_i$ is a motor head's average velocity and $D$ its diffusion coefficient. In the following we choose $D$ to satisfy Einstein's relation when the motor stall force vanishes.

In the following we use $\sqrt{k_BT/k_m}$ as our unit of length, $k_{\text{on}}^0/k_{\text{off}}$ as our unit of probability density and $k_BT$ as our unit of energy. As described in the text, $\eta = \sqrt{k_BT/k_m}/\xi$ is treated as a small parameter. The parameters $\alpha$ and $\beta$ defined in the text are of order $\eta^0$. In our new units, motors have a size $L_m \approx \eta^0$ while filaments sections have a length $\eta^{-1}$.

Denoting by $\boldsymbol{n}_i$ the unit vector of filament $i$ directed towards its barbed end, the position vector of the motor head bound to this filament reads $s_i\boldsymbol{n}_i$ and

$$\begin{aligned}(L_m)^2 &= (s_1\boldsymbol{n}_1 - s_2\boldsymbol{n}_2)^2\\ &= (s_1+s_2)^2\sin^2(\theta/2) + (s_1-s_2)^2\cos^2(\theta/2).\end{aligned} \tag{S5}$$

The longitudinal component of the restoring force exerted on motor head 1 by the spring of constant $k_m$ is

$$f_1^{\|} = -k_m(s_2\boldsymbol{n}_1\cdot\boldsymbol{n}_2 - s_1). \tag{S6}$$

A similar expression holds for head 2.

In the following, we first derive the expressions for the probability density $\rho$ depending on angle $\theta$ and filament coordinates $s_i$. We then combine this result with the dipole exerted by a motor with given $\theta$ and $s_i$ to calculate the average dipole.

*Electronic address: martin.lenz@u-psud.fr

### A. Motor populations

To lowest order in $\eta$, the motor population at the filament ends is negligible and integration of Eq. (S4) yields

$$\rho(\theta) = \iint_{-1/\eta}^{1/\eta} \rho(s_1, s_2; \theta)\, \mathrm{d}s_1\, \mathrm{d}s_2 \underset{\eta\to 0}{\sim} \frac{2\pi}{\sin\theta}. \tag{S7}$$

When $\theta \approx \eta$ or $\pi - \theta \approx \eta$, a fraction of order 1 of each filament's length is within a distance $\approx 1$ of the other filament, and is thus amenable to motor attachment. Conversely, for intermediate $\theta$s, this fraction is of order $\eta$. As a consequence, filaments pairs with $\theta \approx \eta$ or $\pi - \theta \approx \eta$ carry a large fraction of the motor population, and thus $\rho(\theta)$ becomes very large for $\theta$ close to 0 or $\pi$. Defining $u = (s_1 + s_2)/2$ and $v = s_2 - s_1$, we take the successive moments of Eq. (S4) to further compute

$$\langle u \rangle = \frac{\beta}{2[\alpha + \sin^2(\theta/2)]} \tag{S8a}$$

$$\langle u^2 \rangle = \frac{1}{4\sin^2\theta} + \frac{\beta^2}{2[\alpha + \sin^2(\theta/2)][\alpha + 2\sin^2(\theta/2)]} \tag{S8b}$$

$$\langle v \rangle = 0 \tag{S8c}$$

$$\langle v^2 \rangle = \frac{1}{\cos^2(\theta/2)} \tag{S8d}$$

### B. Force dipole

Force balance in Fig. 3(d) yields

$$\mathcal{D}(s_1, s_2; \theta) = -\boldsymbol{f}_1 \cdot \boldsymbol{n}_1 \frac{g(\eta s_1)}{\eta} - \boldsymbol{f}_2 \cdot \boldsymbol{n}_2 \frac{g(\eta s_2)}{\eta}, \tag{S9}$$

with

$$g(S) = \frac{(1-S)^4 - (1+S)^4}{(1-S)^4 + (1+S)^4}. \tag{S10}$$

We average the force dipole exerted by the system over $\theta$ in three dimensions as well as over the attachment-detachment process to find

$$\langle \mathcal{D}_{\text{ext}} \rangle = \frac{\int_0^\pi \iint_{-\xi}^{\xi} \rho(s_1, s_2; \theta) \mathcal{D}(s_1, s_2; \theta)\, \mathrm{d}s_1\, \mathrm{d}s_2\, 4\pi \sin\theta\, \mathrm{d}\theta}{\int_0^\pi \rho(\theta)\, 4\pi \sin\theta\, \mathrm{d}\theta}. \tag{S11}$$

Combining Eqs. (S7) to (S11), we find that the dipole is given by Eq. (10) to lowest order in $\eta$.

## III. DIPOLE GENERATED BY DEFORMABLE FILAMENTS

Here we present a detailed derivation of the filament deformation-induced force dipoles presented in Eqs. (15) and (16) of the main text. We first tackle the small motor force limit $f \ll k_B T \ell_p^{1/2}/\xi^{3/2}$ and derive the average force dipole due to filament bending. We then compute the amount of thermal slack stored in each filament. We use this result to derive the average force dipole in the large-force limit $f \gg k_B T \ell_p^{1/2}/\xi^{3/2}$, where bending becomes irrelevant and filaments are stretched out. Finally, we describe the interpolation between the small- and large-force regimes used in Fig. 4(c)

### A. Dipole in the small-force regime $f \ll k_B T \ell_p^{1/2}/\xi^{3/2}$

We treat the problem pictured in Fig. 4(a) of the main text to compute the force dipole of Eq. (15). Here we give a more detailed treatment than that of Eq. (14) of the main text and include the filaments' stretching energies in our study. These do not modify the scaling of the force dipole but they do have a significant contribution to it. We write the pseudo-energy $E$ of the system in the limit where both the longitudinal strain and the slope $\partial_z x$ of the filament are small (these approximations are justified in the $f \ll k_B T \ell_p^{1/2}/\xi^{3/2}$, $\xi \ll \ell_p$ limit):

$$\begin{aligned} \frac{E}{2} &= \frac{k_B T \ell_p}{2} \int_{-\xi}^{\xi} (\partial_z^2 x)^2\, \mathrm{d}z - f\delta L \\ &+ \frac{k(L+\delta L)}{2} \left\{ \int_{-\xi}^{\delta\ell} \left[1 + (\partial_z x)^2\right] \mathrm{d}z - (L + \delta L) \right\}^2 \\ &+ \frac{k(L-\delta L)}{2} \left\{ \int_{\delta\ell}^{\xi} \left[1 + (\partial_z x)^2\right] \mathrm{d}z - (L - \delta L) \right\}^2 \\ &- \lambda \left[x(\delta\ell) - \delta\ell \tan(\theta/2)\right] \end{aligned} \tag{S12}$$

The first line of Eq. (S12) accounts for the filament bending energy as well as the propensity of the motor to slide towards the barbed end. It is similar to Eq. (14) of the main text, although the term $\delta\ell$ in the motor's pseudo-energy is replaced by $\delta L = L_1^P - \xi$ due to the fact that $\delta\ell \neq \delta L$ for extensible filaments. The second and third lines respectively describe stretching energies of the filament sections proximal to the pointed and barbed ends. As in the main text, we assume that the filament's stretching modulus arises from its bending fluctuations, and thus $k(L) = c k_B T \ell_p^2 / L^4$ with $c$ a numerical constant of order 1. Finally, the fourth of Eq. (S12) enforces the constraint $x(\delta) = \delta\ell \tan(\theta/2)$ through the introduction of the Lagrange multiplier $\lambda$.

We introduce the dimensionless variables

$$\tilde{f} = \frac{f\xi^2}{k_B T \ell_p \tan^2(\theta/2)} \tag{S13a}$$

$$\tilde{x}(\tilde{z}) = \frac{k_B T \ell_p \tan(\theta/2) x(z)}{f\xi^3} \tag{S13b}$$

$$\tilde{z} = \frac{z}{\xi} \quad a = \frac{\delta\ell}{\xi} \quad b = \frac{\delta L - \delta\ell}{\xi} \quad d = \frac{\xi - L}{\xi} \tag{S13c}$$

$$\tilde{\lambda} = \frac{\tan(\theta/2)\lambda}{f} \quad \tilde{k}(\tilde{L}) = \epsilon \frac{\xi^3 k(L/\xi)}{k_B T \ell_p \tan^2(\theta/2) \tilde{f}}. \tag{S13d}$$

In the regime considered here, $\epsilon = f\xi^3/(k_BT\ell_p^2)$ is a small parameter; we also assume small filament stretching: $d \ll 1$. We successively minimize $\tilde{E}$ with respect to $b$ (which imposes longitudinal force balance on the filaments), $\tilde{x}(\tilde{z})$ with boundary conditions $\tilde{x}(-1) = \tilde{x}(1) = \partial_{\tilde{z}}^2\tilde{x}(-1) = \partial_{\tilde{z}}^2\tilde{x}(1) = 0$ (which imposes transverse force balance on the filaments), and $a$ (which fixes the position of the motor along the filament). The minimized energy reads

$$E \simeq \frac{f^2\xi^2}{80k_BT}\frac{a^2(1-a^2)^2(3-a^2)^2}{(1+a^2)^2}, \tag{S14}$$

where $a \in [0,1]$ is the solution of

$$\frac{6a(1+a^2)}{(1-a^2)^3} = \tilde{f}. \tag{S15}$$

In Eq. (S14), the constant $c$ was chosen so as to recover the classic stretching modulus $90k_BT\ell_p^2/(2L)^4$ of a filament of arclength $2L$ in the limit $f \to 0$.

To evaluate the force dipole exerted by the system on the outside medium, we consider an infinitesimal transformation whereby the four anchoring points of the two-filament, one-motor system are displaced radially by a quantity $\mathrm{d}\xi$. This is equivalent to performing the transformation $\xi \to \xi + \mathrm{d}\xi$ while holding $L$ and $\theta$ constant. The work required for this transformation reads

$$\begin{aligned} \mathrm{d}W &= \boldsymbol{f}_1^B \cdot (\boldsymbol{n}_1\mathrm{d}\xi) + \boldsymbol{f}_1^P \cdot (-\boldsymbol{n}_1\mathrm{d}\xi) \\ &\quad + \boldsymbol{f}_2^B \cdot (\boldsymbol{n}_2\mathrm{d}\xi) + \boldsymbol{f}_2^P \cdot (-\boldsymbol{n}_2\mathrm{d}\xi) \\ &= \frac{\mathcal{D}\mathrm{d}\xi}{\xi}, \end{aligned} \tag{S16}$$

where $\boldsymbol{n}_1$, $\boldsymbol{n}_2$ are defined in the previous section. Thus $\mathcal{D}_{\text{bend}}$ can be calculated by differentiating the minimized energy $E$:

$$\begin{aligned} \mathcal{D}_{\text{bend}} &= -\xi\frac{\partial E}{\partial \xi}(k_BT, \ell_p, \xi, L, \theta) \\ &= -\frac{3f\ell_p}{2}\frac{a(1-a^2)(3-a^2)}{1+a^2}. \end{aligned} \tag{S17}$$

Since $a$ depends in $\tilde{f}$ [Eq. (S15)] and $\tilde{f}$ depends on $\theta$, the dipole of Eq. (S17) depends on $\theta$. Averaging it over all values of $\theta$ such that the bent filament length is smaller than the filament arclength (see the section "Interpolation between the small- and large-force regimes" below) and in three dimensions yields Eq. (15) of the main text.

## B. Amount of slack stored in a fluctuating filament

Here we compute the value of the excess length $s$ illustrated in Fig. 4(b) of the main text. We consider an inextensible, three-dimensional worm-like chain with excess length $s$ clamped in $z = -\xi$ and $z = +\xi$ and calculate the associated prestress. Since the filaments of the main text have vanishing prestress in the absence of motors, the correct value of $s$ is then computed by imposing that this prestress be zero.

We parametrize the filament shape by its transverse displacement $\{x(z), y(z)\}$. This filament is almost straight in the $\xi \ll \ell_p$ limit used here, justifying a small angle approximation $\partial_z x \approx \partial_z y \ll 1$. The filament thus has bending a energy

$$\mathcal{H}(x,y) = \frac{k_BT\ell_p}{2}\int_{-\xi}^{\xi}\left[(\partial_z^2 x)^2 + (\partial_z^2 y)^2\right]\mathrm{d}z \tag{S18}$$

and its excess length can be expressed as

$$\mathcal{S}(x,y) = \frac{1}{2}\int_{-\xi}^{\xi}\left[(\partial_z x)^2 + (\partial_z y)^2\right]\mathrm{d}z. \tag{S19}$$

The filament's partition function is thus given by the functional integral

$$Z(s) = \iint \left\{e^{-\mathcal{H}(x,y)/k_BT}\delta\left[\mathcal{S}(x,y) - s\right]\right\}\mathcal{D}x\,\mathcal{D}y, \tag{S20}$$

where the $\delta$ function imposes the predetermined value of the excess length. We introduce the dimensionless variables

$$\tilde{z} = \frac{\pi}{\xi}z, \quad \tilde{s} = \frac{\pi^2\ell_p}{\xi^2}s, \quad \tilde{x}(\tilde{z}) = \frac{\pi\ell_p^{1/2}}{\xi^{3/2}}x(z), \quad \tilde{y}(\tilde{z}) = \frac{\pi\ell_p^{1/2}}{\xi^{3/2}}y(z) \tag{S21}$$

and denote the dimensionless form of the partition function by $\tilde{Z}$. Imposing that $\tilde{x}(\tilde{\xi})$, $\tilde{y}(\tilde{z})$ and their first derivatives vanish at the anchoring points, we compute the Laplace transform

$$\hat{Z}(\sigma) = \int_0^{+\infty} e^{-\sigma\tilde{s}}\tilde{Z}(\tilde{s})\,\mathrm{d}\tilde{s} = \frac{\hat{Z}(0)\pi\sqrt{\sigma}}{\cosh(\pi\sqrt{\sigma})\sinh(\pi\sqrt{\sigma})}. \tag{S22}$$

Inverting the Laplace transform, we find

$$\tilde{Z}(\tilde{s}) = \partial_{\tilde{s}}\left[\vartheta_4\left(e^{-\tilde{s}/4}\right)\right], \tag{S23}$$

where $\vartheta_4$ is the Jacobi theta function [? ].

Finally, we impose a vanishing filament prestress, implying that the filament free energy $F = -k_BT\ln Z$ is minimal as a function of its end-to-end length $\xi$:

$$\frac{\partial F}{\partial \xi} = 0 \quad \Leftrightarrow \quad \frac{\partial \ln\tilde{Z}}{\partial \tilde{s}} = 0. \quad \Rightarrow \quad \tilde{s} \simeq 3.62221. \tag{S24}$$

Combining this result with Eq. (S21) gives the value of $s$.

## C. Dipole in the large-force regime $f \gg k_BT\ell_p^{1/2}/\xi^{3/2}$

Here we derive the average force dipole given in Eq. (16) of the main text and valid for large motor forces and deformable filaments. In this regime, each filament

is assimilated to an inextensible string of arclength $2\xi + s$ and negligible bending modulus attached in two points separated by a distance $2\xi$ as illustrated by the dark filament in Fig. 4(b) of the main text. We label the barbed end of this filament by $B$, the pointed end by $P$ and the motor by $M$. Thus $BP$ denotes the distance between barbed and pointed end and $\widehat{BMP}$ is the angle the filament makes at the point of contact with the motor. Defining $A = [1 + s/(2\xi)]^2$ with $s$ the excess length calculated in the previous section, we use filament length conservation $BM + MP = 2\xi + s$ and the fact that the motor lies on a line at an angle $\theta/2$ with the average filament orientation to find

$$\frac{PM\cos\left(\widehat{BPM}\right)}{\xi} = 1 + \cos(\theta/2)\sqrt{\frac{A(A-1)}{A-\cos^2(\theta/2)}} \tag{S25a}$$

$$\frac{BM\cos\left(\widehat{PBM}\right)}{\xi} = 1 - \cos(\theta/2)\sqrt{\frac{A(A-1)}{A-\cos^2(\theta/2)}} \tag{S25b}$$

$$\frac{PM\sin\left(\widehat{BPM}\right)}{\xi} = \frac{BM\sin\left(\widehat{PBM}\right)}{\xi} \tag{S25c}$$

$$= \sin(\theta/2)\sqrt{\frac{A(A-1)}{A-\cos^2(\theta/2)}} \tag{S25d}$$

We now consider the tension of the filament on either side of the motor. The motor stall condition as described by Eq. (6) of the main text implies a force discontinuity $f^B - f^P = f$, where $f^B$ and $f^P$ are the tensions of the filament sections proximal to the barbed and pointed end, respectively. Additionally, force balance along the horizontal axis of Fig. 4(b) yields

$$f^B\cos\left(\theta - \widehat{PBM}\right) = f^P\cos\left(\theta - \widehat{BPM}\right). \tag{S26}$$

Combining these results with Eqs. (S25) and Eq. (1) of the main text, we find

$$\mathcal{D}_{\text{stretch}}(\theta) = -2f\xi\frac{\left[\sin^2(\theta/2) - (A-1)^2\right]\cos(\theta/2)}{(A-1)^{1/2}[A-\cos^2(\theta/2)]^{3/2}}. \tag{S27}$$

Finally, we average the force dipole over angle in three dimensions for $s \ll 2\xi$ to find

$$\langle\mathcal{D}_{\text{stretch}}\rangle \underset{(A-1)\ll 1}{\sim} -\frac{2\pi f\sqrt{\xi\ell_p}}{\sqrt{\tilde{s}}}, \tag{S28}$$

which yields Eq. (16) of the main text.

### D. Interpolation between the small- and large-force regimes

To interpolate between the dipoles of Eqs. (15) and (16), we use an approximate filament force-extension relation that assumes linear elasticity as long as the filament end-to-end length is shorter than its arclength $2\xi + s$ and inextensibility for higher forces. For a given stall force, filaments are more stretched at small angles $\theta$ than at large angles. Therefore, here the force dipole is given by Eq. (S27) for $\theta < \theta^*$ with $\theta^* = \pi f\xi^{3/2}/[k_BT(30\tilde{s}\ell_p)^{1/2}]$ and by Eq. (S17) for $\theta \geqslant \theta^*$. To lowest order in $\xi/\ell_p$, this yields:

$$\langle\mathcal{D}_{\text{bend \& stretch}}\rangle = \frac{2f\sqrt{\xi\ell_p}}{\sqrt{\tilde{s}}}\sin\theta^* - \frac{3f^2\xi^2}{16k_BT}\ln\frac{\pi}{2\theta^*}, \tag{S29}$$

which is plotted as a black line in Fig. 4(c). Equation (S29) is valid for $\theta^* < \pi/2$ and yields Eq. (15) for $f \ll k_BT\ell_p^{1/2}/\xi^{3/2}$ (or equivalently $\theta^* \ll 1$). For $\theta^* \geqslant \pi/2$, we simply have $\langle\mathcal{D}_{\text{bend \& stretch}}\rangle = \langle\mathcal{D}_{\text{stretch}}\rangle$.

## IV. SENSITIVITY ANALYSIS

To demonstrate that the results presented in Fig. 5 do not depend strongly on the particular choice of parameter values presented in the main text, we monitor the changes in the diagram upon a five-fold change (either upwards or downwards) of each of the following parameters:

- myosin head spacing $l_m$
- myosin head stall force $f_0$
- myosin head duty ratio $1 - p_d$
- typical myosin mechanochemical cycle duration $\tau_d$
- myosin thick filament stretching modulus $\mu$
- myosin unloaded velocity $v_0$.

The results, presented in Fig. S1, show that the regimes of Fig. 5 are remarkably robust even upon these dramatic changes in parameter values.

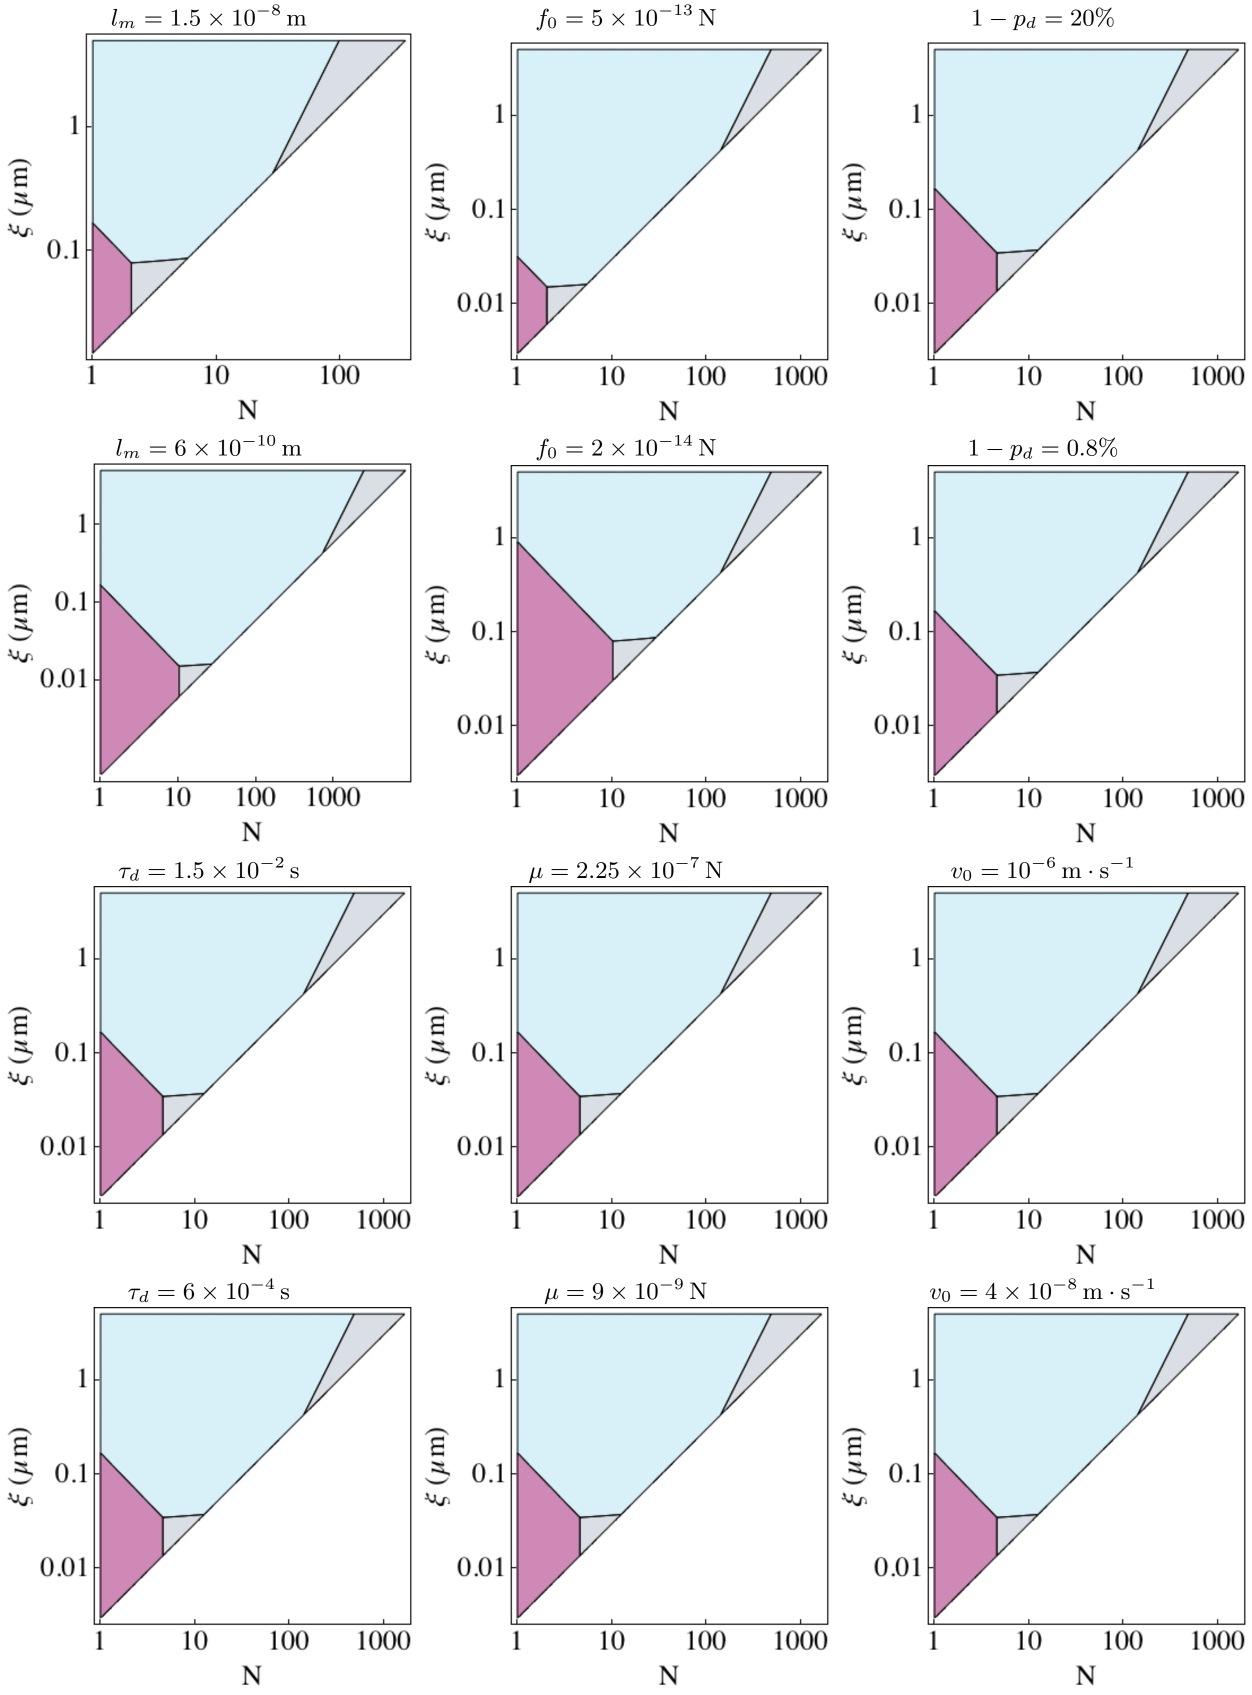


Figure S1: Sensitivity analysis for the regime diagram of Fig. 5 of the main text. Colors are as in the main text, and the position-dependent stall force mechanism never dominates. All parameters are as in the main text except for the one indicated above each panel.
